# Supplementary material for: First-principles study on luminescence properties of Eu-doped defect pyrochlore oxide KNbWO$_6\cdot$H$_2$O:Eu$^{3+}$
Source: arXiv:2001.02059 source file (2019-12-24)
Supplement: Supplementary file 1 [file pyrochlore-supp.pdf]

# Supporting Information – First-principles study on luminescence properties of defect pyrochlore $KNbWO_6 \cdot H_2O{:}Eu^{3+}$

Song-Hyok Choe[a], Chol-Jun Yu[a*], Myong Choe[a], Yun-Hyok Kye[a], Yong-Nam Han[b] and Guangsheng Pang[c]

[a]*Chair of Computational Materials Design, Faculty of Materials Science, Kim Il Sung University, Ryongnam-Dong, Taesong District, Pyongyang, Democratic People's Republic of Korea*

[b]*Faculty of Chemistry, Kim Il Sung University, Ryongnam-Dong, Taesong District, Pyongyang, Democratic People's Republic of Korea*

[c]*State Key Laboratory of Inorganic Synthesis and Preparative Chemistry, College of Chemistry, Jilin University, Changchun 130012, P. R. China*

## Structural model

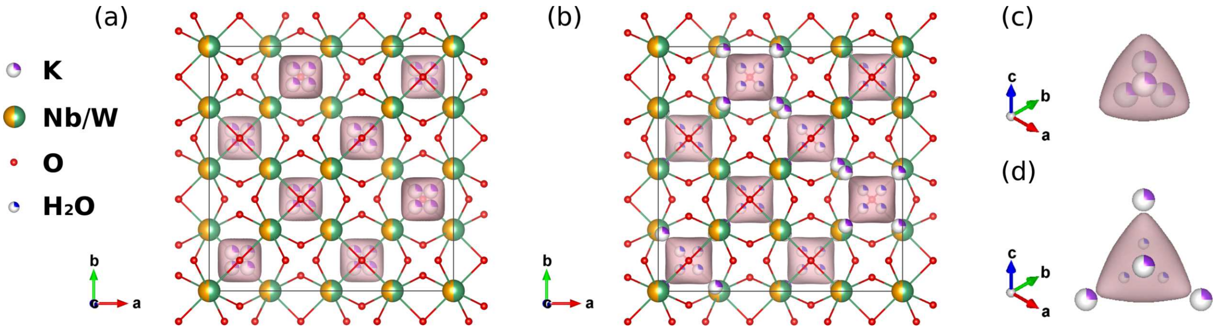


Figure S1. Experimentally determined crystalline structures of (a) $KNbWO_6$ and (b) $KNbWO_6 \cdot H_2O$. BVS isosurfaces are illustrated by light pink surfaces and tetrahedron-like hollow spaces in $KNbWO_6$ and $KNbWO_6 \cdot H_2O$ are shown in (c) and (d), respectively.

*Corresponding author: Chol-Jun Yu, Email: cj.yu@ryongnamsan.edu.kp

## Structural properties

Table S1. Lattice constants ($a$, $b$, $c$), unit cell volume and total energy difference in several structural models for $KNbWO_6 \cdot H_2O$ (Hyd), $KNbWO_6$: $0.125Eu^{3+}$ (Dop) and $KNbWO_6 \cdot H_2O$: $0.125Eu^{3+}$ (HydDop).

| Model | Lattice constant (Å) | | | Volume | $\Delta E$ |
|---|---|---|---|---|---|
| | $a$ | $b$ | $c$ | (Å$^3$) | (meV/atom) |
| $KNbWO_6 \cdot H_2O$ (Hyd) | | | | | |
| Hyd-1 | 10.51 | 10.54 | 10.37 | 1148.01 | 1.39 |
| Hyd-2 | 10.51 | 10.52 | 10.39 | 1149.33 | 0.09 |
| Hyd-3 | 10.51 | 10.48 | 10.42 | 1148.05 | 1.04 |
| $KNbWO_6$: $0.125Eu^{3+}$ (Dop) | | | | | |
| Dop-1-1 | 10.37 | 10.40 | 10.40 | 1121.14 | 0.94 |
| Dop-1-2 | 10.38 | 10.39 | 10.35 | 1116.10 | 3.94 |
| Dop-1-3 | 10.37 | 10.37 | 10.42 | 1120.83 | 4.09 |
| Dop-2-1 | 10.37 | 10.42 | 10.37 | 1121.34 | 0.91 |
| Dop-2-2 | 10.38 | 10.33 | 10.36 | 1111.31 | 0.00 |
| Dop-2-3 | 10.35 | 10.41 | 10.40 | 1120.63 | 3.23 |
| Dop-3-1 | 10.45 | 10.35 | 10.35 | 1120.11 | 3.43 |
| Dop-3-2 | 10.35 | 10.38 | 10.38 | 1114.33 | 2.92 |
| Dop-3-3 | 10.55 | 10.29 | 10.29 | 1117.38 | 24.88 |
| $KNbWO_6 \cdot H_2O$: $0.125Eu^{3+}$ (HydDop) | | | | | |
| HydDop-1 | 10.44 | 10.46 | 10.43 | 1138.23 | 2.09 |
| HydDop-2 | 10.45 | 10.50 | 10.39 | 1138.72 | 0.00 |

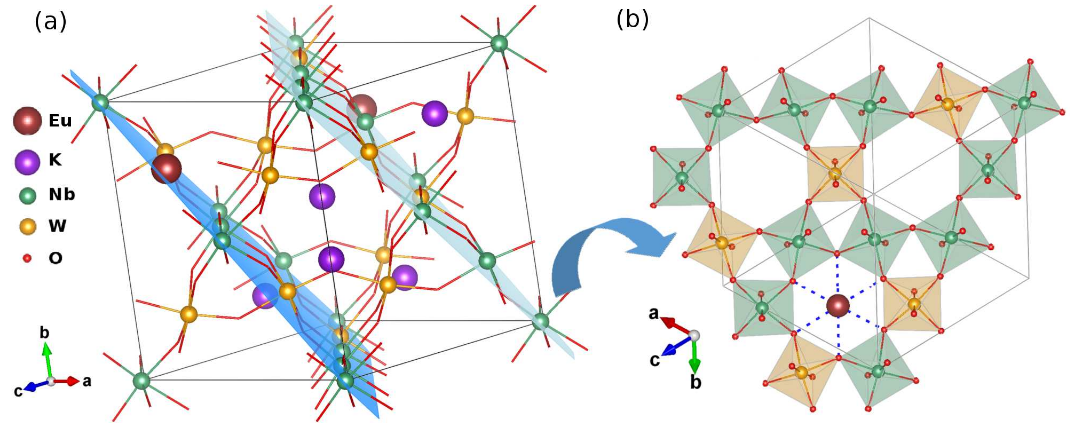


Figure S2. (a) Ball-and-stick view of optimized $KNbWO_6$: $0.125Eu^{3+}$ (Dop) structure with $(1, 1, -1)$ planes designated as light blue planes, and (b) polyhedral view of Nb/W atoms on $(1, 1, -1)$ plane where $Eu^{3+}$ locates.

## Electronic structure

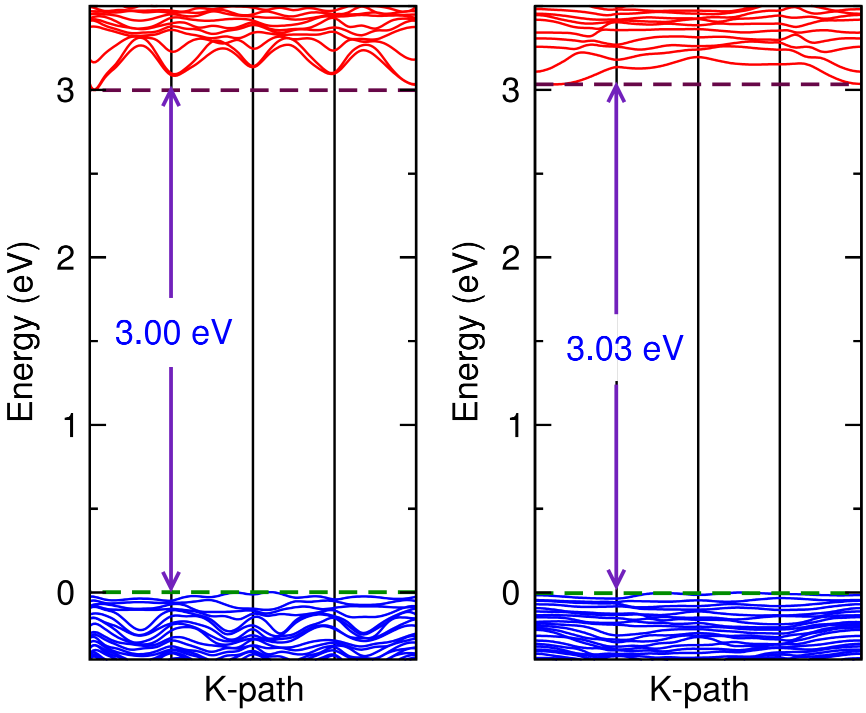


Figure S3. Energy band structure of (a) defect pyrochlore oxide $KNbWO_6$ (Orig) and (b) hydrated defect pyrochlore oxide $KNbWO_6 \cdot H_2O$ (Hyd), calculated by PBEsol + $U$ method. Only spin-up bands are shown.

## Effect of oxygen vacancies

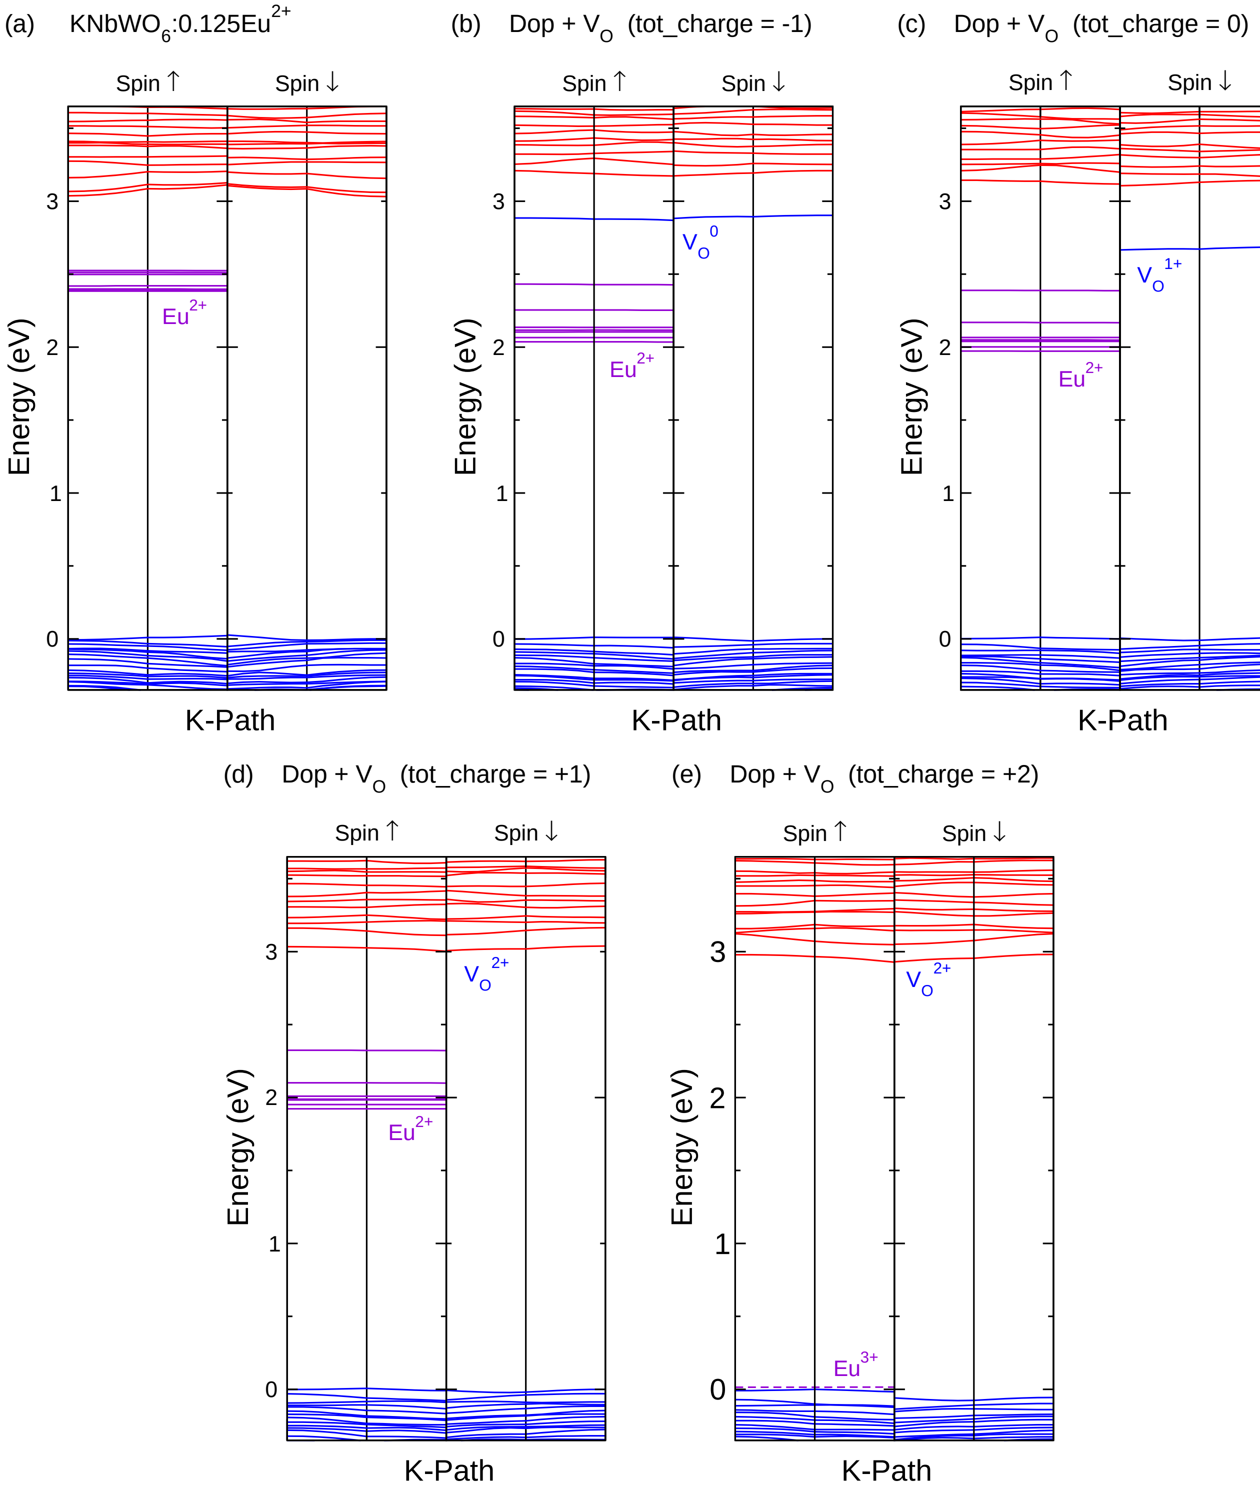


Figure S4. Energy band structure of (a) $KNbWO_6$: $0.125Eu^{2+}$ and $KNbWO_6$: $0.125Eu^{3+}$ with oxygen vacancies (Dop + $V_O$ model) with various total charges of (b) −1, (c) 0, (d) +1 and (e) +2.
